# Supplementary material for: Robust Shift-and-Invert Preconditioning: Faster and More Sample Efficient Algorithms for Eigenvector Computation
Source: arXiv:1510.08896 source file (2016-05-30)
Supplement: Supplementary file 1 [file appendix.tex]

\section{Technical Lemmas}

\subsection{Linear System Facts}
\label{sec:linear-system-facts}

Let $\ma\in\R^{d\times d}$ be a positive definite matrix and consider
\[
f(x) = \frac{1}{2} x^{\top} \ma x - b^{\top} x\,.
\]
Also let
\[
\vx_{*}=\argmin_{\vx}f(\vx)\,.
\]
Now clearly $\grad f(\vx)=\ma\vx-\vb$ and by the optimality of $\vx_{*}$
we have that $\ma x_{*}- b = 0$. Thus we also see that 
\begin{align*}
f(\vx)-f(\vx_{*}) & =\frac{1}{2}\vx^{\top}\ma\vx-\vb^{\top}\vx-\frac{1}{2}\vx^{\top}\ma\vx_{*}+\vb^{\top}\vx_{*}\\
& =\frac{1}{2}\vx^{\top}\ma\vx-\vx_{*}^{\top}\ma\vx+\frac{1}{2}\sum_{i\in[n]}\vx_{*}^{\top}\ma\vx_{*}\\
& =\frac{1}{2}\left(\vx-\vx_{*}\right)^{\top}\ma\left(\vx-\vx_{*}\right)
\end{align*}
Now
\[
\grad f(\vx)=\ma\vx-\vb=\ma\left(\vx-\vx_{*}\right)
\]
